# Supplementary material for: Ultrasensitivity without conformational spread: A mechanical origin for non-equilibrium cooperativity in the bacterial flagellar motor
Source: arXiv:2502.03290 ancillary file (2025-02-05)
Supplement: Supplementary file 1 [file motor_SI.pdf]

# Supporting Information for: Ultrasensitivity without conformational spread: A mechanical origin for non-equilibrium cooperativity in the bacterial flagellar motor

Henry H. Mattingly<sup>1,\*</sup> and Yuhai Tu<sup>2,†</sup>

<sup>1</sup>*Center for Computational Biology, Flatiron Institute, New York, NY, USA*

<sup>2</sup>*IBM Thomas J. Watson Research Center, Yorktown Heights, NY, USA*

(Dated: February 4, 2025)

## I. MECHANICAL MODEL DETAILS

We first construct a simple mechanical model of motor rotation. As described in the main text, we make several simplifying assumptions. First, we assume the motor operates in the over-damped limit and neglect fluctuations. Next, focusing on the stators, we assume that ion refueling and release are fast, so that stator rotation is limited by relaxation down a potential landscape [1, 2].

The torque balance on the stator engaged with the  $i$ 'th FliG subunit is:

$$-\tau_0 + \tau_i(t) - \xi \omega_i(t) = 0. \quad (1)$$

Here,  $\tau_0$  is the slope of the (assumed linear) potential landscape driving stator rotation.  $\tau_i(t)$  is the load torque on the stator from the rotor, and thus is also the output torque exerted by the stator on the rotor.  $\xi$  is the drag on stator rotation, and  $\omega_i(t)$  is the instantaneous rotation velocity of the stator. Since the output torque at  $\omega_i = 0$  is  $\tau_i = \tau_0$ ,  $\tau_0$  is the stator stall torque. Furthermore,  $\omega_0 = \tau_0/\xi$  is the stator rotation speed at zero load. The minus sign in front of  $\tau_0$  above was chosen so that, in the absence of an external load, the stators rotate CW ( $\omega_i < 0$ ). This in turn sets the sign of the opposing load torque, of magnitude  $\tau_i$ .

Next, we assume that FliG subunits have strong interactions with their associated stators, so that the two move at the same translational speed at their point of contact, like gears. We also assume that the rotor rotates as a rigid object. With these, we get the following equation relating the rotation speeds of a stator,  $\omega_i(t)$ , to that of the rotor,  $\Omega(t)$ :

$$r(-\sigma_i(t))\omega_i(t) = R\Omega(t). \quad (2)$$

---

\* [hmattingly@flatironinstitute.org](mailto:hmattingly@flatironinstitute.org)

† [yuhai@us.ibm.com](mailto:yuhai@us.ibm.com)

Here,  $r$  is the radius of a stator and  $R$  is the radius of the C-ring rotor. Including  $\sigma_i(t)$  on the left-hand side allows bi-directional rotation of the C-ring without changes in stator rotation direction [3, 4]. The minus sign in front of  $\sigma_i$  sets  $\sigma_i = -1$  as the FliG conformation that contributes to CW motor rotation. We neglect changes in the radius  $R$  of the C-ring associated with the different FliG conformations.

Plugging Eq. (2) into Eq. (1), using  $1/\sigma_i = \sigma_i$ , multiplying through by  $-1$ , and solving for the stator load torque,  $\tau_i$ , gives:

$$\begin{aligned}\tau_0 - \tau_i(t) - \sigma_i(t) \xi \frac{R}{r} \Omega(t) &= 0 \\ \tau_i(t) &= \tau_0 - \sigma_i(t) \xi \frac{R}{r} \Omega(t) \\ \tau_i(t) &= \tau_0 \left( 1 - \sigma_i(t) \frac{\Omega(t)}{\Omega_0} \right),\end{aligned}\tag{3}$$

where  $\Omega_0 = \frac{\tau_0}{\xi} \frac{r}{R} = \omega_0 \frac{r}{R}$  is the zero-load rotation speed of the rotor.

An immediate and profound consequence of Eq. (3) is that the local torque on a FliG subunit depends both on its own conformation,  $\sigma_i(t)$ , and on the global rotation state of the rotor,  $\Omega(t)$ . In particular, if a FliG subunit's conformation is misaligned with the direction of rotation, then  $\sigma_i(t)$  and  $\Omega(t)$  will have different signs, causing the FliG to experience a large torque. Furthermore, since  $\tau_i \geq 0$  always acts opposite the stator torque in the absence of external motor driving.

Finally, a torque balance on the rotor gives:

$$\sum_{i=1}^N e_i(t) \sigma_i(t) \tau_i(\sigma_i(t)) = \Xi \Omega(t),\tag{4}$$

where  $\Xi$  is the rotational drag on the rotor, and terms in the sum are only nonzero for FliG subunits that are engaged with stators,  $e_i = 1$ . Plugging Eq. (3) into Eq. (4), and using  $\sigma_i^2 = 1$  and conservation of stators:

$$\begin{aligned}\sum_{i=1}^N e_i(t) \sigma_i(t) \tau_0 \left( 1 - \sigma_i(t) \frac{\Omega(t)}{\Omega_0} \right) &= \Xi \Omega(t), \\ \sum_{i=1}^N e_i(t) \left( \sigma_i(t) - \frac{\Omega(t)}{\Omega_0} \right) &= \frac{\Xi \Omega_0}{\tau_0} \frac{\Omega(t)}{\Omega_0}, \\ \sum_{i=1}^N e_i(t) \sigma_i(t) - M \frac{\Omega(t)}{\Omega_0} &= \beta \frac{\Omega(t)}{\Omega_0}.\end{aligned}\tag{5}$$

Above,  $\beta = \Xi \Omega_0 / \tau_0$  is the dimensionless rotational drag on the rotor and  $M$  is the number of

stators. Solving for the rotor rotation velocity gives:

$$\begin{aligned}\frac{\Omega(t)}{\Omega_0} &= \frac{M/\beta}{1 + M/\beta} \frac{1}{M} \sum_{i=1}^N e_i(t) \sigma_i(t) \\ &= \frac{M/\beta}{1 + M/\beta} \left( \frac{N_e^+(t)}{M} - \frac{N_e^-(t)}{M} \right) \\ &= \frac{M/\beta}{1 + M/\beta} \left( 2 \frac{N_e^+(t)}{M} - 1 \right).\end{aligned}\tag{6}$$

Here, we have introduced  $N_e^\pm(t)$ , the number of stator-engaged FliG subunits that are in the conformation  $\sigma = \pm 1$ . In the last line, we again used conservation of stators,  $N_e^+(t) + N_e^-(t) = M$ . Maximum rotation speed is achieved when all FliG subunits are in alignment,  $N_e^+ = 0$  or  $N_e^+ = M$ .

With this, we can express the local torque on a FliG subunit in terms of the global motor state,  $N_e^+$ :

$$\tau_i(t) = \tau_0 \left( 1 - \sigma_i(t) \frac{M/\beta}{1 + M/\beta} \left( 2 \frac{N_e^+(t)}{M} - 1 \right) \right),\tag{7}$$

Thus, the local torque on a FliG subunit depends on whether it is in alignment with the majority. In the main text, we choose units where  $\tau_0 = 1$  and  $\Omega_0 = 1$ . We also define  $\tau_\pm = \tau_i(\sigma_i(t) = \pm 1)$ , which is the same for all engaged subunits in a given conformation,  $\sigma$ .

Eqns. (3) and (7) predict that the magnitude of the load torque on a stator,  $\tau_i$ , can exceed its stall torque,  $\tau_0$ . This occurs when the stator's associated FliG is in the minority conformation, and thus misaligned with the direction of rotation. In this case, the stator is overpowered by the torques applied by other stators on the C-ring. As a result, Eqn. (1) implies that this stator will rotate *counter-clockwise*, the opposite of its usual rotation direction (see Fig. 1 below).

Finally, the torque measured in experiments and used to construct torque-speed curves (as in e.g. [5–7]) is the motor's *output* torque. This is the total net torque applied to the rotor (left-hand side of Eqn. (4)), which equals the drag torque resisting rotation (right-hand side of Eqn. (4)). Assuming that measured motors operate near full alignment  $N_e^+ = 0$  or  $M$ , the measured output torque is:

$$|\tau_{\text{out}}| = \left| \sum_{i=1}^M \tau_i \right| = M \left( 1 - \frac{M/\beta}{1 + M/\beta} \right) = \frac{M}{1 + M/\beta} = \beta |\Omega|.\tag{8}$$

Eliminating the rotational drag,  $\beta$ , gives the predicted (dimensionless) torque-speed curve:

$$|\tau_{\text{out}}| = M (1 - |\Omega|).\tag{9}$$

This linear torque-speed curve resembles the one measured during CW motor rotation [6]. Even when the microscopic mechanics give rise to an output torque-speed curve with a nonlinear shape,

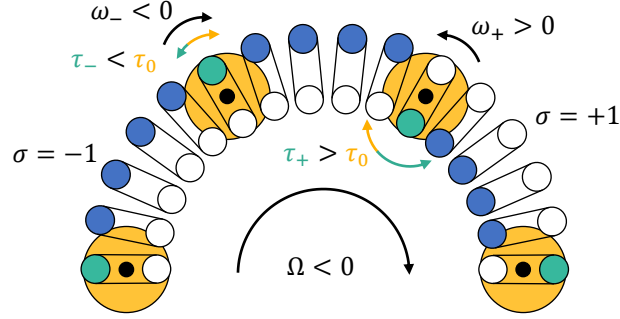

FIG. 1. Zoomed-in schematic of the motor from Fig. 1A of the main text. Here, half of the subunits are shown at a moment in time, and we consider a case where the motor is rotating CW ( $\Omega < 0$ ). Stator-engaged FliG subunits in the conformation  $\sigma = -1$  are in the majority (e.g. the subunit in the upper-left part of the ring). These subunits exert a torque of magnitude  $\tau_- < \tau_0$  on their associated stators (and experience an equal and opposite torque), where  $\tau_0$  is the stall torque produced by the stator. The associated stators rotate with angular velocity  $\omega_- < 0$ , which is aligned with the direction of torque applied by the stator. Net zero torque on the stator is achieved by rotational drag, which acts opposite the direction of stator rotation. Stator-engaged FliG subunits in the opposite conformation,  $\sigma = +1$ , are in the minority (e.g. the subunit in the upper-right part of the ring). These subunits exert a torque of magnitude  $\tau_+ > \tau_0$  on their associated stators (and experience an equal and opposite torque). The associated stators rotate with angular velocity  $\omega_+ > 0$ , which is *opposite* the direction of torque applied by the stator. Thus, assuming strong stator-FliG coupling, this model predicts that some stators transiently rotate in the CCW direction, due to torques from other stators that are transduced through the C-ring.

as in CCW motor rotation, we expect that the local torques experienced by FliG subunits in the majority versus minority conformations will still be different.

## II. CONFORMATION DYNAMICS

Next, we specify the dynamics of FliG conformation changes. FliG's that are unengaged with a stator,  $e_i = 0$ , can undergo the following transitions:

$$\begin{aligned} \sigma_i(t) = -1 &\xrightarrow{k_-} \sigma_i(t) = +1 \\ \sigma_i(t) = +1 &\xrightarrow{k_+} \sigma_i(t) = -1, \end{aligned} \tag{10}$$

where

$$k_{\pm} = k_0 \exp(\mp \Delta F/2). \tag{11}$$

Here,  $\Delta F$  is the free energy preference for the  $\sigma = +1$  conformation, and  $k_0$  is the conformation

transition rate when  $\Delta F = 0$ .  $\Delta F$  includes the effective energetic difference between the two conformations due to CheYp binding.

Stator-engaged FliG subunits,  $e_i = 1$ , undergo conformation changes with modified rates that depend on the local torque that each subunit experiences:

$$k_{\pm}^e = k_{\pm} f(\tau_{\pm}), \quad (12)$$

where  $f(\tau_{\pm})$  is the factor by which the switching rates are enhanced or suppressed as a function of the local torque, which we assume to be a monotonic function of  $\tau$ . Throughout, we will take

$$f(\tau) = \exp(\gamma \tau), \quad (13)$$

with  $\tau$  rescaled by  $\tau_0$ .

In simulations with nearest neighbor coupling (Fig. 4 of the main text), the conformation switching rates in Eqn. (11) were modified to depend on the index (position) of subunit  $i$ :

$$k_{\pm}^i = k_0 \exp\left(\mp \frac{1}{2} (\Delta F + J(\sigma_{i-1} + \sigma_{i+1}))\right), \quad (14)$$

where  $J$  is the energetic coupling between neighboring subunits.

### III. MICROSCOPIC SIMULATION AND ANALYSIS

Stochastic simulations of the motor model above were performed using the Gillespie stochastic simulation algorithm [8]. Conformation transitions above were simulated in the standard way.

In addition to the conformation transitions, rotation was treated as a possible transition. As in Ref. [9], with rate  $\Omega/\Delta\theta$ , the rotor undergoes a rotation event that causes a change of rotor angular position of  $\Delta\theta = \text{sgn}(\Omega(t)) 2\pi/(NM)$  [10–12]. Here,  $2\pi/N$  is the angle between FliG subunits on the C-ring, and  $\text{sgn}(x) \in \{-1, +1\}$  gives the sign of  $x$ . Thus, the timing of rotation events was stochastic, but the direction was deterministic.

Stators were spaced uniformly along the ring of FliG subunits. Stator-subunit exchange upon rotation was treated as follows. First, each stator was labeled with an index  $j \in \{0, \dots, M-1\}$ . Stators would then sequentially take turns exchanging FliG subunits with each step of motor rotation. The stator labeled  $j = 1$  was the first to exchange its FliG subunit upon a rotation event. If the direction of rotation was the same as in the previous rotation event, then stator  $j + \text{sgn}(\Omega(t))$  (modulo  $M$ ) was designated as the next stator to undergo an exchange upon the next rotation event. Otherwise, stator  $j$  remained the designated stator to undergo the next exchange. This

ensured that the spacing between stators was, on average, constant in time. In this scheme, all stators were in contact with a subunit at all times, consistent with the high duty ratio of the motor [5, 12]. Since we assumed each stator interacts with only one FliG subunit, having one stator exchange its subunit a time is important for coordination of subunit conformations in GMC.

Transition paths in Fig. 2B of the main text were computed as follows [13, 14]. The microscopic simulation trajectory (a collection of  $N$  values of  $\sigma$  and  $M$  values of  $e$  at each time point) was projected onto the two-dimensional subspace  $(N_e^+, N_u^+)$  at each time point. Two basins were defined as  $N_e^+ = 0$  and  $N_e^+ = M$ . From the coarse-grained trajectory, we extracted every trajectory segment that left one basin and entered the other basin without returning to the first. Time along each of these transition trajectories was normalized to lie between 0 and 1 and discretized.  $(N_e^+, N_u^+)$  were computed as a function of normalized transition time in the discretization. Finally, averaging  $(N_e^+, N_u^+)$  over transition trajectories at each value of normalized transition time gave the transition path. This was done separately in each direction.

Dissipation rates were calculated from simulation trajectories as in Ref. [15]:

$$\dot{W} = \lim_{T \rightarrow \infty} \frac{1}{T} \sum_{j=1}^{N_T-1} \ln \left( \frac{k_j}{k_j^R} \right) \quad (15)$$

where  $T$  is the trajectory duration,  $N_T$  is the number of transitions,  $k_j$  is the rate of the  $j$ 'th transition, and  $k_j^R$  is the rate of its microscopic reverse transition. Importantly, only transitions associated with conformational dynamics of the  $\sigma_i$  were included in this calculation, since rotation and exchange events were irreversible.

To compute response speeds in Fig. 4 of the main text, microscopic simulations were initiated at  $\Delta F = 1/2$  with all spins in the  $\sigma = +1$  conformation. After allowing the system to relax for  $T = 100 k_0^{-1}$ , the bias was instantaneously changed to  $\Delta F = -1/2$ . Then, the time it took the system to reach  $N_e^+ = 0$  was recorded.  $\tau_R$  was defined to be the average “hit” time of 100 replicate simulations for each parameter set.

#### IV. COARSE-GRAINED MODEL

Since local torques and motor rotation velocity only depend on  $N_e^+$ , this motivates deriving a coarse grained model for the macrostates  $N_e^+$  and  $N_u^+$ , where  $N_u^+$  is the number of unengaged FliG subunits in the conformation  $\sigma = +1$ . Due to conservation of stators, we have  $N_e^+ + N_e^- = M$ , where  $N_e^-$  is the number of engaged subunits in the conformation  $\sigma = -1$ . Furthermore, due to conservation of subunits, we also have  $N_u^+ + N_u^- = N - M$ , where  $N_u^-$  is the number of unengaged

subunits in the conformation  $\sigma = -1$ .

The subunit conformation switching dynamics can be captured exactly with these coarse-grained variables. For unengaged subunits, any one of the  $N_u^-$  subunits in conformation  $\sigma = -1$  can independently transition to conformation  $\sigma = +1$ , causing  $N_u^+$  to increase by 1. Similarly, any one of the  $N_u^+$  subunits can independently transition to the conformation  $\sigma = -1$ , causing  $N_u^+$  to decrease by 1. Thus, in the coarse-grained description, the transitions in Eqn. (10) become:

$$\begin{aligned} N_u^+ &\xrightarrow{(N-M-N_u^+)k_-} N_u^+ + 1 \\ N_u^+ &\xrightarrow{N_u^+k_+} N_u^+ - 1. \end{aligned} \quad (16)$$

Likewise, we have the following conformation transitions among stator-engaged subunits:

$$\begin{aligned} N_e^+ &\xrightarrow{(M-N_e^+)k_- f(\tau_-(N_e^+))} N_e^+ + 1 \\ N_e^+ &\xrightarrow{N_e^+k_+ f(\tau_+(N_e^+))} N_e^+ - 1 \end{aligned} \quad (17)$$

Exchange of stator-associated FliG's requires knowledge of the ring structure, so these transitions must be approximated in the coarse-grained model. First, we assume that one stator exchanges its FliG subunit every time the rotor rotates a distance  $\Delta\theta = 2\pi/(NM)$ , as above. This exchange occurs with rate  $\Omega(N_e^+)/\Delta\theta$ . When this happens, one stator is chosen uniformly at random to disengage with its subunit, and it becomes engaged with a previously unengaged subunit that is also chosen uniformly at random. Exchange transitions are treated as independent processes. These processes can result in two possible transitions in the coarse-grained macro state. One possibility is that an engaged subunit in conformation  $\sigma = -1$  disengages (with probability  $1 - N_e^+/M$ ) and is replaced by a subunit in conformation  $\sigma = +1$  (with probability  $N_u^+/(N - M)$ ), thus increasing  $N_e^+$  by 1 and decreasing  $N_u^+$  by 1. Alternatively, an engaged subunit in conformation  $\sigma = +1$  can disengage (with probability  $N_e^+/M$ ) and be replaced by a subunit in conformation  $\sigma = -1$  (with probability  $1 - N_u^+/(N - M)$ ), thus decreasing  $N_e^+$  by 1 and increasing  $N_u^+$  by 1. Thus, we get the following macroscopic transitions:

$$\begin{aligned} N_e^+, N_u^+ &\xrightarrow{\omega_-(N_e^+, N_u^+)} N_e^+ + 1, N_u^+ - 1 \\ N_e^+, N_u^+ &\xrightarrow{\omega_+(N_e^+, N_u^+)} N_e^+ - 1, N_u^+ + 1. \end{aligned} \quad (18)$$

with rates

$$\begin{aligned} \omega_-(N_e^+, N_u^+) &= \frac{\Omega(N_e^+)}{\Delta\theta} \left(1 - \frac{N_e^+}{M}\right) \frac{N_u^+}{N - M} \\ \omega_+(N_e^+, N_u^+) &= \frac{\Omega(N_e^+)}{\Delta\theta} \frac{N_e^+}{M} \left(1 - \frac{N_u^+}{N - M}\right). \end{aligned} \quad (19)$$

These approximate transitions rates miss correlations between neighboring subunits due to the ring structure. In particular, consider the case where the motor undergoes coherent rotation in either direction, so that the typical duration of a CW or CCW interval is much larger than 1. Subunits that recently disengaged from a stator tend to be aligned with the current direction of rotation. Therefore, the subunits that have been disengaged longest have had the most time to relax and lose memory of the rotation direction. These subunits are also the ones that are most likely to encounter and engage with a stator during coherent rotation. As a result, for a given value of  $N_u^+$ , subunits that newly engage with the stators are more likely to be in the conformation that is *unaligned* with the current rotation direction. The effect of this correlation on the exchange transition rates would be to decrease  $\omega_-(N_e^+, N_u^+)$  (and increase  $\omega_+(N_e^+, N_u^+)$ ) when  $N_e^+ > M/2$ , and vice versa when  $N_e^+ < M/2$ . The transition rates above in Eqn. (19) are good approximations when  $k_0 \gg 1$ , because in this limit the subunits rapidly relax after disengaging from a stator.

With these transitions, the dynamics of the coarse grained model follow a master equation for the joint distribution  $P(N_e^+, N_u^+)$ . It is convenient to write the master equation in terms of operators that step up/down an argument of a function  $f$  by 1:

$$\begin{aligned} E_e^\pm f(N_e^+, N_u^+) &= f(N_e^+ \pm 1, N_u^+) \\ E_u^\pm f(N_e^+, N_u^+) &= f(N_e^+, N_u^+ \pm 1). \end{aligned} \tag{20}$$

We'll use a convention where the operator acts on all terms to its right when there is a product, e.g.  $E_e^\pm f(N_e^+, N_u^+) g(N_e^+, N_u^+) = f(N_e^+ \pm 1, N_u^+) g(N_e^+ \pm 1, N_u^+)$ . Then, the master equation is:

$$\begin{aligned} \partial_t P(N_e^+, N_u^+) &= (E_u^+ - 1) k_+ N_u^+ P(N_e^+, N_u^+) + (E_u^- - 1) k_- (N - M - N_u^+) P(N_e^+, N_u^+) \\ &\quad + (E_e^+ - 1) k_+ f(\tau_+(N_e^+)) N_e^+ P(N_e^+, N_u^+) \\ &\quad + (E_e^- - 1) k_- f(\tau_-(N_e^+)) (M - N_e^+) P(N_e^+, N_u^+) \\ &\quad + (E_e^+ E_u^- - 1) \omega_+(N_e^+, N_u^+) P(N_e^+, N_u^+) \\ &\quad + (E_e^- E_u^+ - 1) \omega_-(N_e^+, N_u^+) P(N_e^+, N_u^+). \end{aligned} \tag{21}$$

### A. Stationary distribution of $N_e^+$

From the master equation in Eqn. (21), we can derive the stationary distribution of  $N_e^+$ . At stationarity, the time derivative on the left-hand side is zero. Then, we need to marginalize out  $N_u^+$  by summing. Since  $P(N_e^+, N_u^+)$  is defined to be zero outside the allowed range of  $N_u^+$ , i.e.  $N_u^+ \in 0, 1, \dots, N - M$ , we can take the sum over  $N_u^+$  from  $-\infty$  to  $\infty$ . We also note that the sum



over step operators can be simplified by shifting the arguments in the infinite sum by 1, as follows:

$$\sum_{N_u^+ = -\infty}^{\infty} E_u^{\pm} f(N_u^+) = \sum_{N_u^+ = -\infty}^{\infty} f(N_u^+ \pm 1) = \sum_{N_u^+ = -\infty \pm 1}^{\infty \pm 1} f(N_u^+) = \sum_{N_u^+ = -\infty}^{\infty} f(N_u^+). \quad (22)$$

Thus, marginalizing over  $N_u^+$  eliminates the shift operators  $E_u^{\pm}$ .

Summing Eqn. (21) over  $N_u$  at stationarity and using the steps in Eqn. (22) above, the first two transitions associated with conformation changes of unengaged subunits all cancel out. The next two transitions associated with conformation changes of engaged subunits don't depend on  $N_u^+$ , so the sum marginalizes out  $N_u^+$  from  $P(N_e^+, N_u^+)$ . In the last two terms, the step operators  $E_u^{\pm}$  disappear. This gives:

$$\begin{aligned} 0 = & (E_e^+ - 1) k_+ f(\tau_+(N_e^+)) N_e^+ P(N_e^+) + (E_e^- - 1) k_- f(\tau_-(N_e^+)) (M - N_e^+) P(N_e^+) \\ & + (E_e^+ - 1) \sum_{N_u^+ = -\infty}^{\infty} \omega_+(N_e^+, N_u^+) P(N_e^+, N_u^+) + (E_e^- - 1) \sum_{N_u^+ = -\infty}^{\infty} \omega_-(N_e^+, N_u^+) P(N_e^+, N_u^+), \end{aligned} \quad (23)$$

where  $P(N_e^+) = \sum_{N_u^+ = -\infty}^{\infty} P(N_e^+, N_u^+)$  is the stationary marginal distribution of  $N_e^+$ . Furthermore, writing  $P(N_e^+, N_u^+) = P(N_u^+ | N_e^+) P(N_e^+)$ , this can be simplified further in terms of averages with respect to the conditional distribution  $P(N_u^+ | N_e^+)$ :

$$\begin{aligned} 0 = & (E_e^+ - 1) k_+ f(\tau_+(N_e^+)) N_e^+ P(N_e^+) + (E_e^- - 1) k_- f(\tau_-(N_e^+)) (M - N_e^+) P(N_e^+) \\ & + (E_e^+ - 1) \langle \omega_+(N_e^+, N_u^+) | N_e^+ \rangle P(N_e^+) + (E_e^- - 1) \langle \omega_-(N_e^+, N_u^+) | N_e^+ \rangle P(N_e^+), \end{aligned} \quad (24)$$

To solve for  $P(N_e^+)$ , we follow the steps in Ref. [16] for stationary solutions of master equations in one variable. First, we group terms in this equation into transitions that increase  $N_e^+$ ,  $t^+(N_e^+)$ , and those that decrease it,  $t^-(N_e^+)$ :

$$\begin{aligned} 0 = & E_e^+ t^-(N_e^+) P(N_e^+) - t^+(N_e^+) P(N_e^+) - (t^-(N_e^+) P(N_e^+) - E_e^- t^+(N_e^+) P(N_e^+)) \\ = & (E_e^+ - 1) J(N_e^+), \end{aligned} \quad (25)$$

where

$$\begin{aligned} t^-(N_e^+) &= k_+ f(\tau_+(N_e^+)) N_e^+ + \langle \omega_+(N_e^+, N_u^+) | N_e^+ \rangle \\ t^+(N_e^+) &= k_- f(\tau_-(N_e^+)) (M - N_e^+) + \langle \omega_-(N_e^+, N_u^+) | N_e^+ \rangle. \end{aligned} \quad (26)$$

In Eqn. (25), we also defined the net flux from  $N_e^+$  to  $N_e^+ - 1$ ,  $J(N_e^+) = t^-(N_e^+) P(N_e^+) - E_e^- t^+(N_e^+) P(N_e^+)$ .

At the left boundary where  $N_e^+ = 0$ , there is no net flux to  $N_e^+ = -1$  since  $t^-(0) = 0$  and  $P(-1) = 0$ . Therefore,  $J(0) = 0$ . Then, summing Eqn. (25) from  $N_e^+ = 0$  to some finite  $N_e^+ - 1$

gives:

$$0 = \sum_{z=0}^{N_e^+-1} (J(z+1) - J(z)) = J(N_e^+) - J(0), \quad (27)$$

and therefore  $J(N_e^+) = 0$  for all  $N_e^+$ . In other words, since this is a one-dimensional system, at stationarity there are no net fluxes across any edges, and the marginalized dynamics obey detailed balance.

Using the definition of  $J(N_e^+)$ , we get  $P(N_e^+) = \frac{t^+(N_e^+-1)}{t^-(N_e^+)} P(N_e^+ - 1)$ , which can be applied recursively to solve the stationary distribution:

$$P(N_e^+) = P(0) \prod_{z=1}^{N_e^+} \frac{t^+(z-1)}{t^-(z)} = \frac{1}{Z} \prod_{z=1}^{N_e^+} \frac{t^+(z-1)}{t^-(z)}, \quad (28)$$

where we replace  $P(0)$  with the normalization constant  $Z = \sum_{N_e^+=0}^M P(N_e^+)$ . Writing this out using the expressions for the stator exchange rates in Eqn. (19), we get:

$$P(N_e^+) = \frac{1}{Z} \prod_{z=1}^{N_e^+} \frac{k_- f(\tau_-(z-1)) (M - (z-1)) + \frac{\Omega(z-1)}{\Delta\theta} (M - (z-1)) \frac{\langle N_u^+ | z-1 \rangle}{N-M}}{k_+ f(\tau_+(z)) z + \frac{\Omega(z)}{\Delta\theta} z \left(1 - \frac{\langle N_u^+ | z \rangle}{N-M}\right)}. \quad (29)$$

Next, both terms in the numerator of the product are proportional to  $M - (z-1)$ , while those in the denominator of the product are proportional to  $z$ . These can be factored out into a separate product that can be simplified:

$$\prod_{z=1}^{N_e^+} \frac{M - (z-1)}{z} = \frac{M!}{N_e^+! (M - N_e^+)!} = \binom{M}{N_e^+}, \quad (30)$$

giving:

$$P(N_e^+) = \frac{1}{Z} \binom{M}{N_e^+} \prod_{z=1}^{N_e^+} \frac{k_- f(\tau_-(z-1)) + \frac{\Omega(z-1)}{\Delta\theta} \frac{\langle N_u^+ | z-1 \rangle}{N-M}}{k_+ f(\tau_+(z)) + \frac{\Omega(z)}{\Delta\theta} \left(1 - \frac{\langle N_u^+ | z \rangle}{N-M}\right)}. \quad (31)$$

Next, we plug in the expressions for conformation switching rates,  $k_{\pm}$ , and  $f(\tau_{\pm})$ , and factor these terms out:

$$\begin{aligned} P(N_e^+) &= \frac{1}{Z} \binom{M}{N_e^+} \prod_{z=1}^{N_e^+} \frac{k_- f(\tau_-(z-1))}{k_+ f(\tau_+(z))} \prod_{z=1}^{N_e^+} \frac{1 + \frac{1}{k_- f(\tau_-(z-1))} \frac{\Omega(z-1)}{\Delta\theta} \frac{\langle N_u^+ | z-1 \rangle}{N-M}}{1 + \frac{1}{k_+ f(\tau_+(z))} \frac{\Omega(z)}{\Delta\theta} \left(1 - \frac{\langle N_u^+ | z \rangle}{N-M}\right)} \\ &= \frac{1}{Z} \binom{M}{N_e^+} \prod_{z=1}^{N_e^+} \exp(\Delta F + \gamma(\tau_-(z-1) - \tau_+(z))) \prod_{z=1}^{N_e^+} \frac{1 + \frac{1}{k_- f(\tau_-(z-1))} \frac{\Omega(z-1)}{\Delta\theta} \frac{\langle N_u^+ | z-1 \rangle}{N-M}}{1 + \frac{1}{k_+ f(\tau_+(z))} \frac{\Omega(z)}{\Delta\theta} \left(1 - \frac{\langle N_u^+ | z \rangle}{N-M}\right)} \\ &= \frac{1}{Z} \binom{M}{N_e^+} \exp\left(\Delta F N_e^+ + \gamma \sum_{z=1}^{N_e^+} (\tau_-(z-1) - \tau_+(z))\right) \prod_{z=1}^{N_e^+} \frac{1 + \frac{1}{k_- f(\tau_-(z-1))} \frac{\Omega(z-1)}{\Delta\theta} \frac{\langle N_u^+ | z-1 \rangle}{N-M}}{1 + \frac{1}{k_+ f(\tau_+(z))} \frac{\Omega(z)}{\Delta\theta} \left(1 - \frac{\langle N_u^+ | z \rangle}{N-M}\right)} \end{aligned} \quad (32)$$

The sum over local torques,  $\tau_{\pm}$ , can be simplified using Eqn. (??):

$$\begin{aligned} \sum_{z=1}^{N_e^+} (\tau_-(z-1) - \tau_+(z)) &= \frac{M/\beta}{1 + M/\beta} \sum_{z=1}^{N_e^+} \left( \left( 2 \frac{z-1}{M} - 1 \right) + \left( 2 \frac{z}{M} - 1 \right) \right) \\ &= -2 \frac{M/\beta}{1 + M/\beta} M \frac{N_e^+}{M} \left( 1 - \frac{N_e^+}{M} \right) \\ &= 2 \frac{M/\beta}{1 + M/\beta} M \left( \left( \frac{N_e^+}{M} - \frac{1}{2} \right)^2 - \frac{1}{4} \right), \end{aligned} \quad (33)$$

where in the last line we completed the square. The additional  $N_e^+$ -independent term introduced by this can be lumped into the normalization constant, so for  $P(N_e^+)$  we now have:

$$P(N_e^+) = \frac{1}{Z} \binom{M}{N_e^+} \exp \left( \Delta F N_e^+ + 2\gamma \frac{M/\beta}{1 + M/\beta} M \left( \frac{N_e^+}{M} - \frac{1}{2} \right)^2 \right) \prod_{z=1}^{N_e^+} \frac{1 + \frac{1}{k_- f(\tau_-(z-1))} \frac{\Omega(z-1)}{\Delta\theta} \frac{\langle N_u^+ | z-1 \rangle}{N-M}}{1 + \frac{1}{k_+ f(\tau_+(z))} \frac{\Omega(z)}{\Delta\theta} \left( 1 - \frac{\langle N_u^+ | z \rangle}{N-M} \right)}. \quad (34)$$

For  $k_0 \gg 1$ , since  $f(\tau_{\pm}) \geq \exp(\gamma) \geq 1$ ,  $k_0 \gg 1$  makes all terms in the product roughly equal 1, to leading order in the small parameter  $1/k_0$ . Then the stationary distribution reduces to:

$$P(N_e^+) = \frac{1}{Z} \binom{M}{N_e^+} \exp \left( \Delta F N_e^+ + 2\gamma \frac{M/\beta}{1 + M/\beta} M \left( \frac{N_e^+}{M} - \frac{1}{2} \right)^2 \right). \quad (35)$$

Finally, as in the main text, we assume  $M/\beta \gg 1$ , giving:

$$P(N_e^+) = \frac{1}{Z} \binom{M}{N_e^+} \exp \left( \Delta F N_e^+ + 2\gamma M \left( \frac{N_e^+}{M} - \frac{1}{2} \right)^2 \right). \quad (36)$$

Lastly, a sum over pairwise energetic couplings among all stator-engaged FliG subunits would be proportional to:

$$\frac{1}{M^2} \sum_{i=1}^N \sum_{j=1}^N e_i \sigma_i e_j \sigma_j = \left( \frac{1}{M} \sum_{i=1}^N e_i \sigma_i \right)^2 = \left( \frac{N_e^+}{M} - \frac{N_e^-}{M} \right)^2 = \left( 2 \frac{N_e^+}{M} - 1 \right)^2 = 4 \left( \frac{N_e^+}{M} - \frac{1}{2} \right)^2, \quad (37)$$

which we identify in the second term of the exponential of Eqn. (36).

As  $\gamma$  gets large, this pairwise coupling term prefers  $N_e^+ \in \{0, M\}$  and penalizes states in between. Thus, the stationary probability of all intermediate states goes to zero, and the distribution over the two remaining states simplifies:

$$P(N_e^+ = M) = \frac{\exp(\Delta F M)}{1 + \exp(\Delta F M)} \quad (38)$$

and  $P(N_e^+ = 0) = 1 - P(N_e^+ = M)$ . This has the form of a Monod-Wymann-Changeux (MWC) model [17], with cooperativity  $M$ . The effects of ligand (CheYp) binding are hidden inside  $\Delta F$ .

### B. Hill coefficient

The stationary average  $\langle N_e^+ \rangle$  is approximately a sigmoidal Hill function of  $\Delta F$ :

$$\frac{\langle N_e^+ \rangle}{M} \approx \frac{\exp(H \Delta F)}{1 + \exp(H \Delta F)}, \quad (39)$$

characterized by Hill coefficient  $H$  [18]. We can derive an approximate Hill coefficient from the relation:

$$\begin{aligned} H &\approx 4 \partial_{\Delta F} \left( \frac{\langle N_e^+ \rangle}{M} \right) \Big|_{\Delta F=0} = \frac{4}{M} \partial_{\Delta F} \left( \sum_{N_e^+=1}^M N_e^+ P(N_e^+) \right) \Big|_{\Delta F=0} \\ &= \frac{4}{M} \left( \sum_{N_e^+=1}^M N_e^+ P(N_e^+) \partial_{\Delta F} \log(P(N_e^+)) \right) \Big|_{\Delta F=0}. \end{aligned} \quad (40)$$

When  $k_0 \gg 1$ , using Eqn. (36),

$$\begin{aligned} H &\approx \frac{4}{M} \left( \sum_{N_e^+=1}^M (N_e^+)^2 P(N_e^+) - \partial_{\Delta F} \log(Z) \sum_{N_e^+=1}^M N_e^+ P(N_e^+) \right) \Big|_{\Delta F=0} \\ &= \frac{4}{M} \left( \langle (N_e^+)^2 \rangle - \langle N_e^+ \rangle^2 \right) \Big|_{\Delta F=0} = \frac{4}{M} \text{Var}(N_e^+) \Big|_{\Delta F=0} \end{aligned} \quad (41)$$

In the second line, we used  $\partial_{\Delta F} \log(Z) = \langle N_e^+ \rangle$ . At zero bias ( $\Delta F = 0$ ), the mean  $N_e^+$  is  $\langle N_e^+ \rangle|_{\Delta F=0} = M/2$ . The maximum variance of  $N_e^+$  is achieved when all weight in  $P(N_e^+)$  is at the extremes  $N_e^+ = 0$  and  $N_e^+ = M$ , with equal weight. In this case, the variance of  $N_e^+$  is  $M^2/2 - (M/2)^2 = M^2/4$ . Thus,  $\text{Var}(N_e^+) \leq M^2/4$ , and  $H \leq M$ .

Using Gillespie simulations of the ring structure, we verify in Fig. 2 that this qualitative result, that  $H$  increases with  $M$ , holds even when there is nearest-neighbor energetic coupling  $J$  between neighboring FliG subunits. Furthermore, nearest-neighbor coupling alone does not result in substantial changes in  $H$  with  $M$ —this requires mechanical coupling, i.e.  $\gamma > 0$ .

### V. FITS TO EXPERIMENTAL MEASUREMENTS OF CW BIAS

We assume that the motor CW bias,  $CW$ , is approximately a Hill function of the average intracellular concentration of CheYp,  $Y$ , as measured previously [21, 22]:

$$CW(Y, K, H) = \frac{(Y/K)^H}{1 + (Y/K)^H}. \quad (42)$$

The half-maximum CheYp concentration,  $K$ , and the Hill coefficient,  $H$ , can in principle depend on the load.

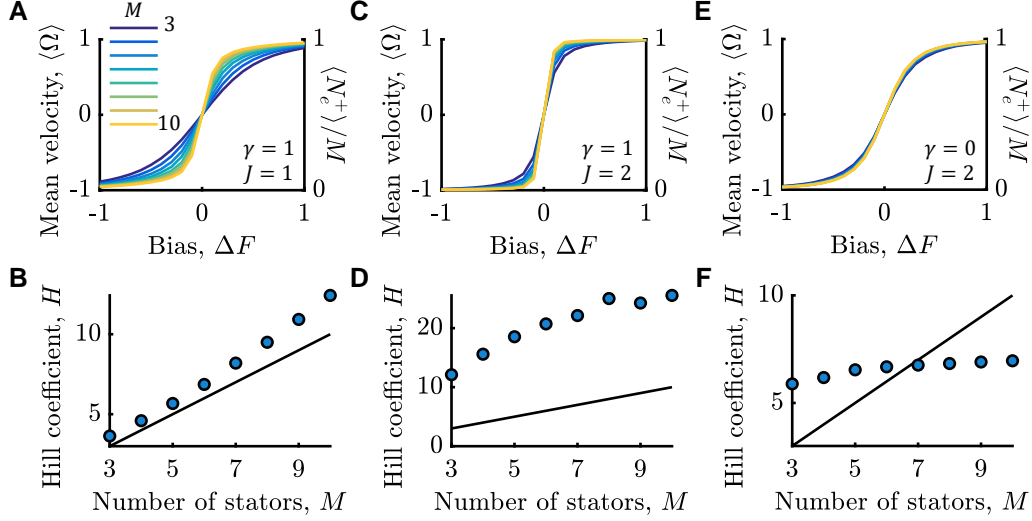

FIG. 2. GMC predicts that the Hill coefficient,  $H$ , increases with stator number  $M$  even when there is nearest-neighbor coupling between FliG subunits,  $J > 0$ . A, C, E) Dose-response curves of average motor angular velocity versus energetic bias for  $\sigma = +1$ ,  $\Delta F$ , for varying values of  $\gamma$  and  $J$ . Colors denote the value of  $M$ , marked in (A). B, D, F) Response Hill coefficient  $H$  versus number of stators  $M$  for the cases above. Black lines show  $y = x$  for reference. (E, F) are essentially the conformational spread model [19, 20], which does not have mechanical coupling ( $\gamma = 0$ ) and does not show substantial changes in  $H$  with  $M$ . We use a smaller value of  $J$  (2 rather than 4 in past works) to show that  $H$  is not flat because of saturation at  $H \leq N$ , but instead genuinely does not depend strongly on  $M$ .

In the experiments performed in Ref. [23], CW bias,  $y_i$  was measured in individual motors  $i$  under multiple load conditions. We focus on data measured using  $0.35 \mu\text{m}$  beads, since roughly half of the motor's stator sites are occupied in aqueous conditions for this bead size [24]. To change the load, the authors added Ficoll to the experimental medium, which increases its viscosity. In these experiments,  $Y_i$  in each cell is unknown, and we assume it does not change with load.

In this model, the unknown parameters are the CheYp concentrations  $\{Y_i\}$  of the  $N$  cells in the data set; the Hill coefficients in 0% and 19% w/v Ficoll,  $H(0\%)$  and  $H(19\%)$  (assumed to be the same for all cells); and the half-maximum CheYp concentrations in the two conditions,  $K(0\%)$  and  $K(19\%)$  (also assumed to be the same for all cells).

These parameters cannot all be uniquely determined from the data available. To see this, we rearrange Eqn. (42):

$$(Y/K)^H = \frac{CW}{1 - CW}. \quad (43)$$

Thus, given a set of measured CW biases in one load condition, different choices of the parameters  $\{Y_i\}$ ,  $H$ , and  $K$  can perfectly compensate each other and produce equally good fits to the data.

To remove this invariance, we first use Eqn. (43) in the two experimental conditions to eliminate  $Y$ , which is assumed to be the same in both:

$$\begin{aligned} CW(19\%) &= \left( \frac{K(0\%)}{K(19\%)} \right)^{H(19\%)} \left( \frac{CW(0\%)}{1 - CW(0\%)} \right)^{H(19\%)/H(0\%)} \\ &= B \left( \frac{CW(0\%)}{1 - CW(0\%)} \right)^A, \end{aligned} \quad (44)$$

where arguments denote the concentration of Ficoll. Assuming the measurements of CW bias in each condition are noisy, a minimal set of structurally-identifiable model parameters is the  $N$  “true” but unobserved CW biases in 0% Ficoll,  $CW_i(0\%)$ , together with the parameters  $A$  and  $B$ .

For ease of comparison with previous works, we perform a different fit with the same number of parameters. To break in the invariances of Eqn. (43), as in Ref. [23], we fix  $H(19\%) = 10.3$  and  $K(19\%) = 3.1\mu\text{M}$ , which are the values of  $H$  and  $K$  measured in Ref. [21]. Then, the unknown parameters are the CheYp concentrations in each cell,  $\{Y_i\}$ , and the Hill function parameters in 0% Ficoll,  $H(0\%)$  and  $K(0\%)$ . Although the inferred values of these parameters are contingent on the assumed values of  $H(19\%)$  and  $K(19\%)$ , the corresponding inferred values of  $\{CW_i(0\%)\}$ ,  $A$ , and  $B$  are not. What’s important for our purposes is the relative values of the Hill coefficients in the two load conditions, quantified by  $A$ . For completeness, we also perform fits using the parameterization with  $\{CW_i(0\%)\}$ ,  $A$ , and  $B$ , arriving at similar results.

Assuming Gaussian-distributed measurement uncertainties for cell  $i$  and Ficoll concentration  $c$ ,  $\sigma_i(c)$ , the log-likelihood function is:

$$\mathcal{L} \propto -\frac{1}{2} \sum_{c \in \{0\%, 19\%\}} \sum_{i=1}^N \left( \frac{y_i(c) - CW(Y_i, K(c), H(c))}{\sigma_i(c)} \right)^2, \quad (45)$$

where  $CW(Y_i, K, H)$  is the function in Eqn. (42). We excluded data points in which measured CW bias,  $y_i(c)$ , was below 0.05 or above 0.95. Best-fitting parameters were found by locally minimizing  $\mathcal{L}$  using the Levenberg-Marquardt algorithm [25, 26], implemented by the function *lsqnonlin* in MATLAB (Natick, MA), with initial guesses  $Y_i = K(19\%)$  for all  $i$ ,  $K(0\%) = K(19\%)$ , and  $H(0\%) = H(19\%)$ . To ensure positive parameters, we fit the logarithms of all parameters. Parameter uncertainties were found by Markov-chain Monte Carlo (MCMC) using a custom implementation of the Metropolis-Hastings algorithm [27, 28]. The prior was taken to be uniform over log-parameters.

The inferred Hill function parameters were  $H(0\%) = 6.0 \pm 0.3$ ,  $K(0\%) = 3.24 \pm 0.01\mu\text{M}$ . Uncertainties are the standard deviations of the MCMC samples. The corresponding inferred values of the parameters  $A$  and  $B$  were  $A = 1.7 \pm 0.1$ ,  $B = 1.59 \pm 0.03$ .

In the alternative parameterization where  $Y$  is eliminated, the likelihood function is proportional to:

$$\mathcal{L}_{alt} \propto -\frac{1}{2} \sum_{i=1}^N \left( \frac{y_i(19\%) - CW(CW_i(0\%), A, B)}{\sigma_i(19\%)} \right)^2 - \frac{1}{2} \sum_{i=1}^N \left( \frac{y_i(0\%) - CW_i(0\%)}{\sigma_i(0\%)} \right)^2, \quad (46)$$

where  $CW(CW_i(0\%), A, B)$  is the function in Eqn. (44). Best-fitting parameters and uncertainties were found as above. To ensure that  $CW_i(0\%)$  remained between 0 and 1, we fit the transformed parameter  $b_i = \ln \left( \frac{CW_i(0\%)}{1-CW_i(0\%)} \right) \in (-\infty, \infty)$ . To ensure positivity of  $A$  and  $B$ , we fit the logarithms of these parameters. The prior was taken to be uniform over these transformed parameters. The inferred values of the parameters  $A$  and  $B$  were  $A = 1.70 \pm 0.09$ ,  $B = 1.59 \pm 0.06$ .

- 
- [1] Y. Tu and Y. Cao, Design principles and optimal performance for molecular motors under realistic constraints, [Physical Review E \*\*97\*\*, 022403 \(2018\)](#).
  - [2] Y. Cao, T. Li, and Y. Tu, Modeling Bacterial Flagellar Motor With New Structure Information: Rotational Dynamics of Two Interacting Protein Nano-Rings, [Frontiers in Microbiology \*\*13\*\* \(2022\)](#).
  - [3] M. Santiveri, A. Roa-Eguiara, C. Kühne, N. Wadhwa, H. Hu, H. C. Berg, M. Erhardt, and N. M. I. Taylor, Structure and Function of Stator Units of the Bacterial Flagellar Motor, [Cell \*\*183\*\*, 244 \(2020\)](#).
  - [4] J. C. Deme, S. Johnson, O. Vickery, A. Aron, H. Monkhouse, T. Griffiths, R. H. James, B. C. Berks, J. W. Coulton, P. J. Stansfeld, and S. M. Lea, Structures of the stator complex that drives rotation of the bacterial flagellum, [Nature Microbiology \*\*5\*\*, 1553 \(2020\)](#).
  - [5] W. S. Ryu, R. M. Berry, and H. C. Berg, Torque-generating units of the flagellar motor of *Escherichia coli* have a high duty ratio, [Nature \*\*403\*\*, 444 \(2000\)](#).
  - [6] J. Yuan, K. A. Fahrner, L. Turner, and H. C. Berg, Asymmetry in the clockwise and counterclockwise rotation of the bacterial flagellar motor, [Proceedings of the National Academy of Sciences \*\*107\*\*, 12846 \(2010\)](#).
  - [7] Y. Niu, R. Zhang, and J. Yuan, Flagellar motors of swimming bacteria contain an incomplete set of stator units to ensure robust motility, [Science Advances \*\*9\*\*, eadi6724 \(2023\)](#).
  - [8] D. T. Gillespie, Stochastic Simulation of Chemical Kinetics, [Annual Review of Physical Chemistry \*\*58\*\*, 35 \(2007\)](#).
  - [9] F. Bai, T. Minamino, Z. Wu, K. Namba, and J. Xing, Coupling between Switching Regulation and Torque Generation in Bacterial Flagellar Motor, [Physical Review Letters \*\*108\*\*, 178105 \(2012\)](#).
  - [10] A. D. Samuel and H. C. Berg, Fluctuation analysis of rotational speeds of the bacterial flagellar motor., [Proceedings of the National Academy of Sciences \*\*92\*\*, 3502 \(1995\)](#).
  - [11] A. D. Samuel and H. C. Berg, Torque-generating units of the bacterial flagellar motor step independently, [Biophysical Journal \*\*71\*\*, 918 \(1996\)](#).

- [12] Y. Sowa, A. D. Rowe, M. C. Leake, T. Yakushi, M. Homma, A. Ishijima, and R. M. Berry, Direct observation of steps in rotation of the bacterial flagellar motor, *Nature* **437**, 916 (2005).
- [13] R. Zakine and E. Vanden-Eijnden, Minimum-Action Method for Nonequilibrium Phase Transitions, *Physical Review X* **13**, 041044 (2023).
- [14] D. Hathcock, Q. Yu, and Y. Tu, Time-reversal symmetry breaking in the chemosensory array reveals a general mechanism for dissipation-enhanced cooperative sensing, *Nature Communications* **15**, 8892 (2024).
- [15] Q. Yu and Y. Tu, Energy Cost for Flocking of Active Spins: The Cusped Dissipation Maximum at the Flocking Transition, *Physical Review Letters* **129**, 278001 (2022).
- [16] C. Gardiner, *Stochastic Methods: A Handbook for the Natural and Social Sciences*, 4th ed. (Springer, Berlin, Heidelberg, 2009).
- [17] J. Monod, J. Wyman, and J.-P. Changeux, On the nature of allosteric transitions: A plausible model, *Journal of Molecular Biology* **12**, 88 (1965).
- [18] A. V. Hill, The possible effects of the aggregation of the molecules of haemoglobin on its dissociation curves, *J Physiol* **40**, 4 (1910).
- [19] T. A. J. Duke, N. Le Novère, and D. Bray, Conformational spread in a ring of proteins: a stochastic approach to allostery, *Journal of Molecular Biology* **308**, 541 (2001).
- [20] F. Bai, R. W. Branch, D. V. Nicolau, T. Pilizota, B. C. Steel, P. K. Maini, and R. M. Berry, Conformational Spread as a Mechanism for Cooperativity in the Bacterial Flagellar Switch, *Science* **327**, 685 (2010).
- [21] P. Cluzel, M. Surette, and S. Leibler, An Ultrasensitive Bacterial Motor Revealed by Monitoring Signaling Proteins in Single Cells, *Science* **287**, 1652 (2000).
- [22] J. Yuan and H. C. Berg, Ultrasensitivity of an Adaptive Bacterial Motor, *Journal of Molecular Biology* **425**, 1760 (2013).
- [23] S. Zhu, R. He, R. Zhang, and J. Yuan, Mechanosensitive dose response of the bacterial flagellar motor, *Physical Review E* **110**, 054402 (2024).
- [24] M. J. Tipping, N. J. Delalez, R. Lim, R. M. Berry, and J. P. Armitage, Load-Dependent Assembly of the Bacterial Flagellar Motor, *mBio* **4**, 10.1128/mbio.00551 (2013).
- [25] K. Levenberg, A method for the solution of certain non-linear problems in least squares, *Quarterly of Applied Mathematics* **2**, 164 (1944).
- [26] D. W. Marquardt, An Algorithm for Least-Squares Estimation of Nonlinear Parameters, *Journal of the Society for Industrial and Applied Mathematics* **11**, 431 (1963).
- [27] N. Metropolis, A. W. Rosenbluth, M. N. Rosenbluth, A. H. Teller, and E. Teller, Equation of State Calculations by Fast Computing Machines, *The Journal of Chemical Physics* **21**, 1087 (1953).
- [28] W. K. Hastings, Monte Carlo sampling methods using Markov chains and their applications, *Biometrika* **57**, 97 (1970).
